# Supplementary material for: Higher Order Recurrent Space-Time Transformer for Video Action Prediction
Source: arXiv:2104.08665 source file (2021-09-21)
Supplement: Supplementary file 1 [file 2_analysis.tex]

We don't need to use patches, but the trade-off is we need 3x3 spatial kernels. Assuming we are all using 1x1 kernels, it becomes $8C^2$, which is cheaper than their $12C^2$. Another point is, the ViT based model usually needs several layers, they stack 6 in minimal, and can up to 12 layers. We have recurrent, so more efficient (i.e., accuracy / \#layers) using only with few layers (e.g., we use 2 for anticipation problem and 4 for early recognition on nearly no backbone settings)
